# Supplementary material for: ReZero: Region-customizable Sound Extraction
Source: arXiv:2308.16892 source file (2023-08-31)
Supplement: Supplementary file 1 [file 7_appendix.tex]

\section{APPENDIX: Room Impulse Response Simulation}
The multi-channel room impulse response (RIR) is simulated on-the-fly using fast random simulation of multi-channel RIR (FRAM-RIR) \cite{luo2022fra}. 
The positions of speech sources, microphone array positions, as well as those of the directional interferences (which will be mentioned in \ref{sec:app_noise}), are randomly sampled within the room, with a minimum distance of 0.5 meters from the wall.

\begin{table}[h]
    \caption{The multi-channel RIR simulation configurations for training different ReZERO models. }
    \label{tab:rir}
    \centering
    \begin{tabular}{c|c|c|c}
        \toprule
         \textbf{Model ID} & \textbf{Room size (m, L-W-H)} & \textbf{$T_{60}$} & \textbf{SNR (dB)} \\
         \midrule
         G & $[3,3,2.5] - [8,6,4]$ & 0.05 - 0.7 & \\         
         \hline
         \#1 & \\
         \hline
         \#2 &  \\
         \hline
         \#3 & $[5,5,3] - [12,10,4]$  & 0.05 - 0.4 & \\
        \bottomrule
    \end{tabular}
\end{table}

\section{APPENDIX: Noise Simulation}
\label{sec:app_noise}
To make the simulation more realistic, we consider three types of noises in the simulation pipeline to train and validate the proposed model. %The noise simulation contributes to the overall performance. 

\textbf{Directional noise}. The directional interference comes from a specific direction, such as knocking, tapping, music and fan noise. The position of the directional interference is randomly sampled and the multi-channel RIR is accordingly simulated based on the room size, $T_{60}$, and position information. The noise signal is convolved with the multi-channel RIR to form the directional noise. 

% \textbf{Additive noise}.
\textbf{Isotropic noise}. Isotropic noise emits equal power in all directions, which is commonly recognized as “environmental noise”. We adopt \emph{spherical} isotropic noise model based on the implementation in \cite{}. 

\textbf{Babble noise}. Babble noise (multi-speaker noise) is one of the most challenging interference for speech processing models due to its similarity to the desired target speech. In our implementation, the multi-channel babble noise is simulated by adding up separate single-speaker reverberant speech signals. The locations of babble speech signals are randomly sampled within the room, with a minimum speaker-to-array distance of 1.5 meters. 

\begin{table}[h]
    \caption{The configurations for simulating different types of noise. “number” indicates the sampling number range of each noise type for each mixture utterance. }
    \label{tab:babble_noise}
    \centering
    \begin{tabular}{c|c|c|c}
        \toprule
         \textbf{Noise type} & \textbf{Noise data} & \textbf{number} & \textbf{SNR (dB)} \\
         \midrule
         Directional noise & \makecell[c]{DNS-Challenge \cite{}, \\ MUSAN \cite{snyder2015musan}, \\ Nonspeech \cite{hu2010nonspeech}} & $[0, 2]$ & $[6, 15]$ \\
         \hline
         Isotropic noise & Gaussian noise & $[0, 1]$ & $[8, 15]$ \\
         \hline
         Babble noise & LibriSpeech \cite{panayotov2015librispeech} &$[10, 20]$ & $[20, 40]$ \\
        \bottomrule
    \end{tabular}
\end{table}

\section{APPENDIX: Ablation Study on the number of microphone elements}
\label{sec:app_ablation_me}

\section{APPENDIX: Ablation Study on the microphone spacing}
\label{sec:app_ablation_ms}
